# Supplementary material for: On Guillotine Separable Packings for the Two-dimensional Geometric Knapsack Problem
Source: arXiv:2103.09735 source file (2021-03-17)
Supplement: Supplementary file 1 [file Appendix0.tex]

\section{Omitted parts from Sections \ref{sec:intro}, \ref{sec:prelim}, \ref{glp}}
\subsection{Guillotine stages}
\label{subsec:guill} 
We define a {\em stage} of guillotine cuts as a set of end to end, equal, axis-parallel cuts separating piece $P$ into further sub-pieces. A guillotine stage packing  is represented by guillotine stage tree $\mathcal{T}$  where each non-leaf node $v\in V(\mathcal{T})$ is equipped with a piece $P_v$ and the set of straight lines  $\mathcal{L}_v$ corresponding the stage of the  cut such that cutting $P_v$ along the straight lines in $\mathcal{L}_v$ gives us subpieces $P_{v_1}, P_{v_2}, \dots, P_{v_{|\mathcal{L}_v|}}$, where $v_1, v_2, \dots, v_{|\mathcal{L}_v|}$ are the children of $v$. 
None of the guillotine cuts are allowed to cut any of the rectangles in the piece.
Note that two consecutive levels of $\mathcal{T}$ correspond to two different type of stages, one being horizontal (parallel to $x$-axis) cuts and the other being vertical cuts (parallel to $x$-axis).  A guillotine packing strategy  has $k$-stages if the  tree $\mathcal{T}$ has height $k$ (e.g. the guillotine stage tree for the 5-stage packing in \ref{figb} is shown below).

\begin{forest}
[,circle,draw
 [,circle,draw, fill = blue
	 [,circle,draw, fill = red
		 [,circle,draw, fill = green
			 [,circle,draw, fill = brown]
			 [,circle,draw, fill = brown]
		]
		 [,circle,draw, fill = green]
	 ]
	 [,circle,draw, fill = red]
	 [,circle,draw, fill = red]
	 [,circle,draw, fill = red]
	 [,circle,draw, fill = red]
	 [,circle,draw, fill = red
		 [,circle,draw, fill = green]
		 [,circle,draw, fill = green]
		 [,circle,draw, fill = green]
		 [,circle,draw, fill = green
			 [,circle,draw, fill = brown]
			 [,circle,draw, fill = brown]
			 [,circle,draw, fill = brown]
			 [,circle,draw, fill = brown]
		]
	]
 ]
 [,circle,draw, fill = blue
	 [,circle,draw, fill =  red
		 [,circle,draw, fill = green]
		 [,circle,draw, fill = green]
	 ]
	 [,circle,draw, fill =  red
		 [,circle,draw, fill = green]
		 [,circle,draw, fill = green]
	 ]
	 [,circle,draw, fill = red
		 [,circle,draw, fill = green
			 [,circle,draw, fill = brown]
			 [,circle,draw, fill = brown]
			 [,circle,draw, fill = brown]
			 [,circle,draw, fill = brown]
		 ]
		 [,circle,draw, fill = green
			 [,circle,draw, fill = brown
				[,circle,draw, fill = yellow]
				[,circle,draw, fill = yellow]
				[,circle,draw, fill = yellow]
			]
			 [,circle,draw, fill = brown]
		 ]
		 [,circle,draw, fill = green]
	]
 ]
 [,circle,draw, fill = blue
 	[,circle,draw, fill = red
		[,circle,draw, fill = green]
		[,circle,draw, fill = green]
	]
 	[,circle,draw, fill = red
		[,circle,draw, fill = green]
		[,circle,draw, fill = green]
	]
 	[,circle,draw, fill = red]
	[,circle,draw, fill = red
		[,circle,draw, fill = green
			[,circle,draw, fill = brown]
			[,circle,draw, fill = brown]
			[,circle,draw, fill = brown]
		]
		[,circle,draw, fill = green]
		[,circle,draw, fill = green]
		[,circle,draw, fill = green]
		[,circle,draw, fill = green]
		[,circle,draw, fill = green]	
	]
 ]
]
\end{forest}

Now we show that we can check whether a given packing of items in a knapsack is guillotine separable or not. We state the following result:

\begin{lem}
\label{polygil}
Given a packing of $n$ items in a $N\times N$ knapsack, we can verify if it guillotine separable or not in $O(n^{2})$-time.
\end{lem}
\begin{proof}
We first claim that given a set of guillotine separable items, with their end coordinates, there exists an end-to-end guillotine cut passing along the  edge of at least one item, not intersecting any item. This claim trivially follows by considering an end-to-end guillotine cut on the piece and appropriately shifting it to touch edge of the nearest item. Now we devise the following procedure to check if a given packing is guillotine separable or not. Search for an end-to-end guillotine cut along end points of items which leaves us with $4n$ choices ($2n$ each for vertical and horizontal end points of items). If such a cut is obtained, we recurse over the two smaller sub-pieces formed and apply the same procedure. Otherwise, if there is no such possible cut, the algorithm returns a NO instance. The algorithm halts when all the items are on distinct sub-pieces, or if a NO instance is obtained at any recursive step. Clearly this recursive procedure takes $O(n^2)$-time.  
\end{proof}

\subsection{Processing of subcorridor}\label{prosec}
In \cite{adamaszek2015knapsack, GalvezGHI0W17} the subcorridors are processed so that by removing some items the remaining items in that subcorridor can packed into a constant number of boxes.

\begin{lem}
For appropriate constant $\epsb, \eps>0$, given a  boundary-$\Lc$ corridor in a guillotine separable box, we can process one subcorridor and remove two sets of rectangles {\em kill} and {\em thin} and rearrange the remaining rectangles (we call them {\em fat}) such that all fat rectangles are completely packed into $O_{\epsb}(1)$ boxes, $|kill|=O_{\eps, \epsl, \epsb}(1)$ and total area of thin rectangles $\le \epsb N^2$. More over, the packing remains guillotine separable. 
\end{lem}
%\arir{check if it is better to mention the width of thin etc. shift this proof to appendix.}
\begin{proof}
We will use similar {\em processing} as shown in \cite{GalvezGHI0W17}.
W.l.o.g we show the processing for a vertical subcorridor (processing for horizontal subcorridor follows analogous process).
Consider the vertical subcorridor $S_{V}$.
Let the width of the $S_{V}$ be $w$. Divide the region of $S_{V}$ in $1/\epsb$ subregions by introducing vertical lines equally spaced between left and right edges of the subcorridor by a distance of $\epsb w$. Items that are cut by the vertical lines are marked as $kill$. Items in the left-most subregion are marked as $thin$ and the items in the remaining subregions are marked as $fat$ (see Figure \ref{fig:lproc}(a)). 
Clearly, the total area of thin rectangles $\le \epsb N^2$.
Now create a maximal rectangular box in each sub region. Remove the  items marked as $kill$ and $thin$ and shift the remaining items to the boxes in the lower subregions. Consider the boundary curve $C$ of the corridor between $S_V$ and $S_H$, the horizontal subcorridor, as shown in  We then consider the set of points $Q$ on $C$ which are a part of the rectangular boxes created. 
% Let the boundary curve of $S_{3}$ which does not share boundary with $S_{2}$. Let this be $C'$.
Now project the points $Q$ via horizontal lines through the horizontal subcorridor $S_{H}$ until they hit the vertical edge of  $S_{H}$ (see Figure  \ref{fig:lproc}(b)). 
Items that are cut by these horizontal lines are too marked as $kill$. 
As all rectangles in kill have length $\epsl$ in the direction of cut,  $|kill|=O_{\eps, \epsl, \epsb}(1)$.
This ends the procedure of processing as we get $O_{\epsb}(1)$ boxes (see Figure  \ref{fig:lproc}(c)). 
%. Now repeat the same process for $(C',Q')$. 
%The process terminates as the spiral have constant number of bends. 
%The process leads to the formation of corridors with lower number of bends as shown in \ref{fig:lproc}. 
Also by loosing a small profit from the items marked as $fat$ we can find a container packing in polynomial time using Lemma \ref{tool:container}. Let the items packed in the container packing be $\optfa^{cont}$.

Similar procedure can be repeated for processing of horizontal subcorridors. 

Intuitively, one can view the creation of boxes in {\em processing of a subcorridor} as a series of guillotine cuts. 
The rearrangement of boxes can be viewed as movement of subpieces without violating guillotine separability. These movements do not disturb other parts of the bounding box as these cuts do not pass through the rest of the boxes. 
\end{proof}
